# Supplementary material for: TRUST: Triangle Counting Reloaded on GPUs
Source: arXiv:2103.08053 source file (2021-03-14)
Supplement: Supplementary file 1 [file appendix.tex]

\begin{appendices}

\section{Proof of Graph Reordering as NP-complete}\label{sec:proof}
{Analogous to the graph coloring problem (GCP), our graph reordering problem (GRP) for minimizing hash collision is also NP-complete. Particularly, in GCP, a graph $G$ is colored with an objective of minimizing the number of colors ($k$) used to label vertices in $G$ such that each pair of adjacent vertices have different colors~\cite{holyer1981np}. Similarly, in GRP, we determine the ordering of graph which incurs minimum collision with $k$ buckets while
using \textsc{hash}$(v)$ function to place a vertex in a specific bucket of $hashTable$.
%in reordered graph is analogous to labeling a vertex $v$ with a specific color in GCP. 
The constraint of a GCP instance -- two vertices connected by one edge should have different colors -- maps to the constraint of a GRP instance that two vertices belonging to one vertex's $neighborList$ should have different hash value or be mapped to different buckets. We prove that GRP is a NP-complete problem by reducing a GCP instance to a GRP instance.
%To prove GRP is a NP-complete problem, we reduce a GCP instance to a GRP instance.
}

\textbf{Reducing GRP to GCP}. Suppose we have a GCP instance
$\langle G(E,V),k\rangle$ where $k$ is the number of colors. A GRP instance can be defined as $\langle G'(E',V'),\phi,bucketNumber \rangle$ where {$\phi$ is the estimated cost of linear search defined in Equation~(\ref{eq:cost_est})} and $bucketNumber$ represents the number of buckets in the $hashTable$. The reduction process is performed as follows:

Initially, we set $V'=V, E'=\emptyset$. 
%i.e., copy all the vertices from $V$ to $V'$. 
For each edge $(u,v) \in E$, we create a vertex $x_{uv}$ and add it to $V'$. With $x_{uv}$ as a source vertex, we add two directed edges $(x_{uv},u)$ and $(x_{uv},v)$ to $E'$. For each vertex $v_i' \in V'$, we create a new vertex $y_i'$ and add it to $V'$. Again, for each newly created vertex $y_i'$, an edge $(v_i',y_i')$ is generated and added to $E'$. This ensures that the {outdegree} of $v_i'$ and $x_{uv}$ is always equal to 1 and 2, respectively. 
Then, we set {$\textsc{hash}(u)$} as $u\%k$ so that the number of colors in $G'$ equals to the number of hash buckets in $G'$. 
Here, if vertices $u$ and $v$ are assigned the same color in $G$, it means there is a hash collision between vertices $u$ and $v$ in $x_{uv}.neighborList$ of $G'$. Hence, a GCP instance is reduced to a GRP instance. This reduction process can be completed in a polynomial time.

%{\textbf{Reducing GRP to GCP}.  For any GCP instance $\langle G(E,V),k\rangle$, we can convert it into a GRP instance $\langle G'(E',V'),\phi,bucketNumber \rangle$ with the following steps: 1) Let $V'=V, E'=\emptyset$. In graph $G'$, we use $v_i$ to represent the vertices directly copied from $G$. 2) For edge $(u,v) \in E$, we create a vertex $x_{uv}$ and insert it into $V'$. Based on vertex $x_{uv}$, create two edges $(x_{uv},u)$ and $(x_{uv},v)$. In this way, the same color between $u$ and $v$ maps to the hash collision in $x_{uv}.neighborList$. 3) For each vertex $v_i \in V'$, create a new vertex $y_i$, put it into $V'$ then create an edge $(v_i,y_i)$. This step ensures that the degree of $v_i$ is 1 and the collective degree of $x_{uv}$ is 2. 4) Set \textsc{hash} function $\textsc{hash}(u.ID)$ as $u\%k$ so that the number of hash buckets is equal to the number of colors. 5) Add $\text{max}(0,k|V|-2|V|-|E|)$ vertices $z_i$ having zero neighbor into $V'$. Now, $|V'|=\text{max}(k|V|,2|V|+|E|)$ and $|E'|=2|E|+|V|$, so that each hash bucket will have at least $|V|$ vertex IDs. }

%{Since the vertices $y_i$ and $z_i$ do not have any neighbor, the max collision of these vertices are equal to 0 and we can ignore them in $\phi$. Vertices $v_{i}$ do not have 2-hop neighbors, the collective degree of $v_i$ are equal to 0 and we can also ignore them in $\phi$. Now, we only need to consider the collision in $x_{uv}.neighborList$. As we mentioned before, the max collision of $x_{uv}$ is at least 1 and the collective degree of $x_{uv}$ is 2. }

\begin{figure}[hb]
	% \vspace{-0.4cm}
	\centering
    \includegraphics[width=.8\linewidth]{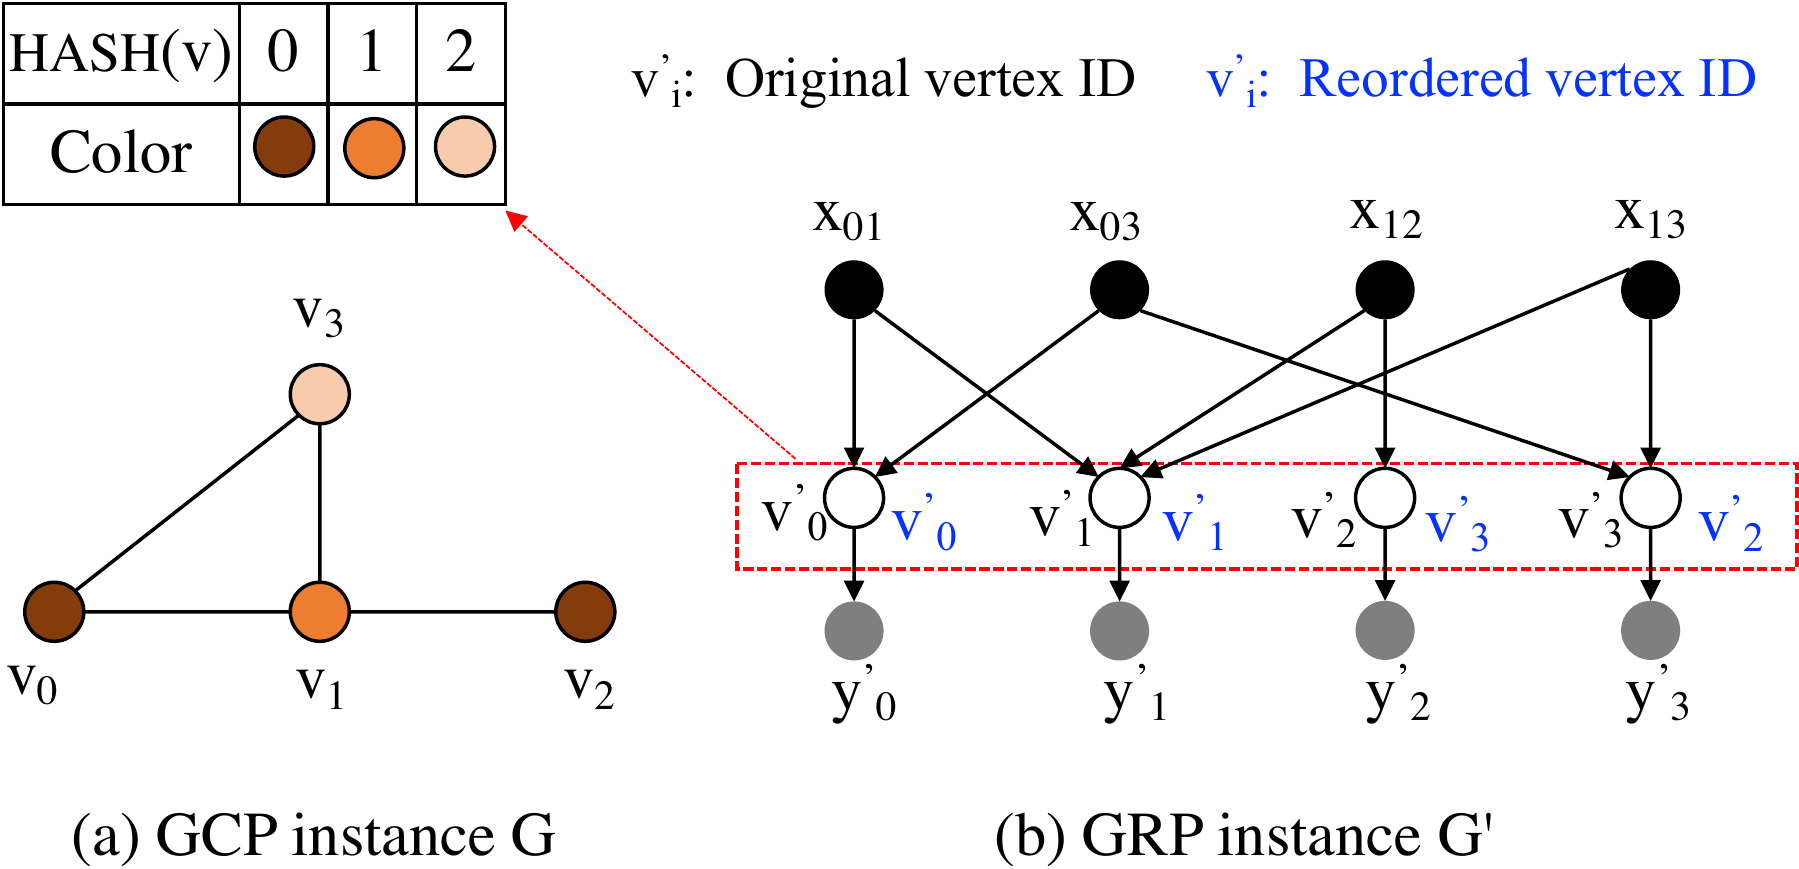}
    
	\vspace{.1in}
	\caption{An example of reducing GRP to GCP.}
	\label{fig:proof}
% 	\vspace{-0.2in}

\end{figure}

\textbf{Example}. {Figure~\ref{fig:proof} shows an example for reducing a GCP instance to a GRP instance. Suppose we want to determine if three distinct colors ($k$=3) can be used for coloring $G$ in 
%For a GCP problem which includes four vertices and four edges in 
Figure~\ref{fig:proof}(a). We follow the reduction steps mentioned earlier to convert it into a GRP instance $G'$ as shown in Figure~\ref{fig:proof}(b). First, let $V'$ = $V$. 
Second, we construct four new vertices $\{x_{01},x_{03},x_{12},x_{13}\}$ and connect them with corresponding $v_i'$ with the edges in $E$. Taking $x_{01}$ as an example, we generate two edges $(x_{01},v_0')$ and $(x_{01},v_1')$ and add them in $E'$.
Third, we add vertices $\{y_0',y_1',y_2',y_3'\}$, as well as the edges from $\{v_0',v_1',v_2',v_3'\}$ to $\{y_0',y_1',y_2',y_3'\}$, respectively. We set the hash function as {$\textsc{hash}(u)=u\%3$}. Here, the number of buckets is equal to the number of distinct colors. 
After $G'$ has been constructed, assume we find a reordering result, i.e., new vertex IDs for vertices in $G'$ as shown in figure~\ref{fig:proof}(b) and ensure no collision exists on $x_{uv}.neighborList$. We use the hash values of reordered vertex IDs (labeled as blue in Figure~\ref{fig:proof} (b)) as color for the vertices in $G$. The ordering of the remaining vertices will not affect the color or the collision in $G'$. We can color $v\in G$ by {$\textsc{hash}(v)$} as shown in Figure~\ref{fig:proof}(a). In this way, a GRP instance can be converted into a GCP instance.}

% \fixme{}

% {Assume we can find an order of GRP that $\phi=2|V|$ in polynomial time so that there is no collision in the $neighborList$ of $x_{uv}$, i.e., for a vertex $x_{uv}\in V'$, \fixme{$\textsc{hash}(u.ID)\neq \textsc{hash}(v.ID)$}. If we assign color given by \fixme{$\textsc{hash}(u.ID)$} function to vertex $u\in V$ for an edge $(u,v) \in E$, the color of $u$ is different from the color of $v$. Since the construction and mapping can also be done in polynomial time, GCP can be solved in polynomial time.}
% Further, if there exists a coloring scheme of GCP, there must exist a reordering answer of GRP. We can assign the vertex $v\in G'$ with a \fixme{$v.ID$ and $\textsc{hash}(v.ID)=v_{color}$}. Then we can assign the rest IDs to the remaining vertices. 

\end{appendices}
